# Supplementary material for: SensorBench: Benchmarking LLMs in Coding-Based Sensor Processing
Source: arXiv:2410.10741 source file (2025-03-28)
Supplement: Supplementary file 1 [file archive_6_Appendix.tex]

\section{Appendix}

\newpage
\newpage

\begin{table*}[ht]
\centering
\resizebox{0.95\textwidth}{!}{%
\begin{tabular}{lrlll}
\toprule
 Task & Tools & Key methodology & Difficulties & Common \\
\midrule
Change point detection & Hybrid & Perform STFT + call API & 4.3 & Y \\
Delay detection & Hybrid + API & Compute Autocorrelation and Crosscorrelation & 3 & Y \\
ECG heartrate  & Hybrid + API & Data cleaning + Peak detection & 2 & Y \\
Echo cancellation & Hybrid & Normalize + autocorrelation + peak detection + adaptive filtering & 4 & Y \\
Extrapolation & Hybrid & Peak detection + Right shift signal by one / multiple peak & 3 & Y \\
Filtering ECG & API + handcraft & lowpass filter FIR & 1.3 & Y and N \\
Filtering Speech & Hybrid & FFT visualization + low pass / high pass filter + binary search (by perceptual feedback) + bandpass filter (eventually) & 3.5 & Y \\
Imputation & Hybrid & Peak detection + Right shift signal by one / multiple peak & 3 & Y \\
Outlier detection & Hybrid or API & Window + meadian filtter + substraction + peak detection & 3 & Y \\
Period detection & API & Autocorrelation & 1 & Y \\
Resampling & API & API & 1 & Y \\

\bottomrule
\end{tabular}

}
\caption{Expert 1's Approaches and Difficulties in Solving the Benchmark}
\label{table:exp-1}
\end{table*}

\subsection{Recovery respiration signal from mmWave Radar}\label{uwb_radar}

The dataset is collected with a SensorLogic SLMX4 UWB radar, which sends repeating pulses to the environment at a center frequency of 7.29 GHz and a bandwidth of 1.4 GHz. As a remote sensing modality, the UWB radar sends pulses reflected on human chests and abdomens to measure their vital signs remotely. The ground truth is provided by a respiration monitor belt sensor Neulog NUL-236 mounted on the chest of the human subject. The UWB radar is controlled by a Raspberry Pi 4B via a serial peripheral interface (SPI) while the ground truth sensor is controlled by a Windows laptop. The system implements Precision Time Protocol (PTP) to ensure we acquire time-synchronized waveforms between the two sensors. We recruited 12 volunteers and instructed them to sit relaxed at a 1.5m distance and to breathe normally. The study is IRB-approved (IRB protocol number omitted for anonymity). In total, we collected a 15-hour dataset of human respiration measured by UWB radar, with time-synchronized ground truth.\looseness=-1

% algorithm
The collected UWB radar is a two-dimension complex time series. The first dimension is time. Sampled at 50~\!Hz, each UWB measurement lasts 30 seconds, resulting in a length of 1500 samples. The second dimension is space (distance). Thanks to the ranging capability of radar, UWB data divides the space ranging from 0.3~\!m to 4.3~\!m in front of the sensor into 120 different bins, each representing a distance range of 5.14~\!cm. At a particular distance and time, the UWB data contains two orthogonal channels, in-phase (I) and quadrature (Q). Conventionally, the I/Q samples are represented as a complex number I+jQ. In short, the UWB data matrix is a complex matrix $\mathbb{M} \in \mathrm{C}^{T \times D}$, where $T$ indicates time and $D$ indicates distance bins. To recover the respiration, a typical signal-processing system (such as the one introduced in \cite{zheng2020v2ifi}) needs to identify the distance bin containing the human subject and take a slice over the spatial dimension to obtain a 1D time series. Then, the system needs to convert the complex time series to real-valued ones by taking the phase, amplitude, real part, or imagery part of the complex numbers. Additional denoising and smoothing algorithms can optionally be applied to the final time series to generate a sequence that best represents human vital signs.

As shown in the code \ref{lst:gpt4o_example}, GPT-4o provides the solver implementation to recover respiration traces. The model use priori knowledge of common respiration rate (from 0.2 to 0.5 Hz) and seak for the bins with the highest power in the corresponding frequency range.

\begin{lstlisting}[language=Python, caption={GPT-4o's solution}, label={lst:gpt4o_example}]
def solver(input_data, sampling_rate):
    radar_matrix_np = input_data
    # Parameters
    sampling_rate = 50  # Hz
    duration = 30  # seconds
    respiration_range = (0.2, 0.5)  # Hz
    # Compute the Fourier Transform for each column
    fft_results = np.zeros((radar_matrix_np.shape[1], radar_matrix_np.shape[0] // 2))
    frequency_bins = fftfreq(radar_matrix_np.shape[0], 1 / sampling_rate)[:radar_matrix_np.shape[0] // 2]

    for col in range(radar_matrix_np.shape[1]):
        column_data = radar_matrix_np[:, col]
        fft_result = fft(column_data)
        fft_magnitude = np.abs(fft_result)[:radar_matrix_np.shape[0] // 2]
        fft_results[col, :] = fft_magnitude

    # Identify the columns with significant power in the respiration frequency range
    respiration_indices = np.where((frequency_bins >= respiration_range[0]) & (frequency_bins <= respiration_range[1]))[0]
    respiration_power = fft_results[:, respiration_indices].sum(axis=1)

    # Find the column with the maximum respiration power
    best_column_index = np.argmax(respiration_power)
    return best_column_index
\end{lstlisting}


\begin{figure*}[htbp]
    \centering

    \begin{subfigure}[b]{0.22\textwidth}
        \includegraphics[width=\textwidth]{./figure/comp_mode/n_Change point detection.png}
        \caption{Change point detection}
        % \label{fig:change_point_detection}
    \end{subfigure}
    \begin{subfigure}[b]{0.22\textwidth}
        \includegraphics[width=\textwidth]{./figure/comp_mode/n_Filtering Speech.png}
        \caption{Spectral filtering-speech}
        % \label{fig:echo_cancellation}
    \end{subfigure}
    \begin{subfigure}[b]{0.22\textwidth}
        \includegraphics[width=\textwidth]{./figure/comp_mode/n_Outlier detection.png}
        \caption{Outlier detection}
        % \label{fig:outlier_detection}
    \end{subfigure}
    \begin{subfigure}[b]{0.22\textwidth}
        \includegraphics[width=\textwidth]{./figure/comp_mode/n_Echo cancellation}
        \caption{Adaptive filtering}
        % \label{fig:filtering_speech}
    \end{subfigure}
    
    \begin{subfigure}[b]{0.22\textwidth}
        \includegraphics[width=\textwidth]{./figure/comp_mode/n_Filtering ECG.png}
        \caption{Spectral filtering-ECG}
        % \label{fig:change_point_detection}
    \end{subfigure}
    \begin{subfigure}[b]{0.22\textwidth}
        \includegraphics[width=\textwidth]{./figure/comp_mode/n_ECG heartrate.png}
        \caption{Heart rate calculation}
        % \label{fig:echo_cancellation}
    \end{subfigure}
    \begin{subfigure}[b]{0.22\textwidth}
        \includegraphics[width=\textwidth]{./figure/comp_mode/n_Resampling.png}
        \caption{Resampling}
        % \label{fig:outlier_detection}
    \end{subfigure}
    \begin{subfigure}[b]{0.22\textwidth}
        \includegraphics[width=\textwidth]{./figure/comp_mode/n_Period detection.png}
        \caption{Period detection}
        % \label{fig:filtering_speech}
    \end{subfigure}
    
    \begin{subfigure}[b]{0.22\textwidth}
        \includegraphics[width=\textwidth]{./figure/comp_mode/n_Delay detection.png}
        \caption{Delay detection}
        % \label{fig:change_point_detection}
    \end{subfigure}
    \begin{subfigure}[b]{0.22\textwidth}
        \includegraphics[width=\textwidth]{./figure/comp_mode/n_Imputation.png}
        \caption{Imputation}
        % \label{fig:echo_cancellation}
    \end{subfigure}
    \begin{subfigure}[b]{0.22\textwidth}
        \includegraphics[width=\textwidth]{./figure/comp_mode/n_Extrapolation.png}
        \caption{Extrapolation}
        % \label{fig:outlier_detection}
    \end{subfigure}


    \caption{Performance comparison with different interaction modes for various tasks. LLMs include GPT-4o, GPT-4 turbo (denoetd as GPT-4), GPT-3.5-turbo (denoetd as GPT-3.5), Llama-3-70b (denoted as Llm-3). Tasks (a) - (d) are evaluated using SDR; thus, the higher the metric, the better the performance. For the remaining tasks, the lower the metric, the better the performance. \xiaomin{(1) what is A, NA, T, should explain in the caption also (2) using more distinct colors (3) I feel that figures are a bit distracted, consider changing to tables.}}
    \label{fig:performance_comparison_mode}
    
\end{figure*}

\begin{figure*}[htbp]
    \centering

    \begin{subfigure}[b]{0.22\textwidth}
        \includegraphics[width=\textwidth]{./figure/comp_N/n_Change point detection.png}
        \caption{Change point detection}
        % \label{fig:change_point_detection}
    \end{subfigure}
    \begin{subfigure}[b]{0.22\textwidth}
        \includegraphics[width=\textwidth]{./figure/comp_N/n_Filtering Speech.png}
        \caption{Spectral filtering-speech}
        % \label{fig:echo_cancellation}
    \end{subfigure}
    \begin{subfigure}[b]{0.22\textwidth}
        \includegraphics[width=\textwidth]{./figure/comp_N/n_Outlier detection.png}
        \caption{Outlier detection}
        % \label{fig:outlier_detection}
    \end{subfigure}
    \begin{subfigure}[b]{0.22\textwidth}
        \includegraphics[width=\textwidth]{./figure/comp_N/n_Echo cancellation}
        \caption{Echo cancellation}
        % \label{fig:filtering_speech}
    \end{subfigure}

        \begin{subfigure}[b]{0.22\textwidth}
        \includegraphics[width=\textwidth]{./figure/comp_N/n_Filtering ECG.png}
        \caption{Spectral filtering-ECG}
        % \label{fig:change_point_detection}
    \end{subfigure}
    \begin{subfigure}[b]{0.22\textwidth}
        \includegraphics[width=\textwidth]{./figure/comp_N/n_ECG heartrate .png}
        \caption{Heart rate calculation}
        % \label{fig:echo_cancellation}
    \end{subfigure}
    \begin{subfigure}[b]{0.22\textwidth}
        \includegraphics[width=\textwidth]{./figure/comp_N/n_Resampling.png}
        \caption{Resampling}
        % \label{fig:outlier_detection}
    \end{subfigure}
    \begin{subfigure}[b]{0.22\textwidth}
        \includegraphics[width=\textwidth]{./figure/comp_N/n_Period detection.png}
        \caption{Period detection}
        % \label{fig:filtering_speech}
    \end{subfigure}

        \begin{subfigure}[b]{0.22\textwidth}
        \includegraphics[width=\textwidth]{./figure/comp_N/n_Delay detection.png}
        \caption{Delay detection}
        % \label{fig:change_point_detection}
    \end{subfigure}
    \begin{subfigure}[b]{0.22\textwidth}
        \includegraphics[width=\textwidth]{./figure/comp_N/n_Imputation.png}
        \caption{Imputation}
        % \label{fig:echo_cancellation}
    \end{subfigure}
    \begin{subfigure}[b]{0.22\textwidth}
        \includegraphics[width=\textwidth]{./figure/comp_N/n_Extrapolation.png}
        \caption{Extrapolation}
        % \label{fig:outlier_detection}
    \end{subfigure}


    \caption{Performance Comparison for Various Tasks. Filtering Speech, Echo cancellation, Change point detection, Outlier detection, and Echo cancellation (the first row) are the larger the better; the remaining tasks are the smaller the better.}
    \label{fig:performance_comparison_diff_n}
    
\end{figure*}
